# Supplementary material for: Dynamic Random Choice
Source: arXiv:2102.00143 source file (2022-06-20)
Supplement: Supplementary file 1 [file 6_SuppApp.tex]

\subsection{Proof of Corollary 2, Forwards Direction}


\subsection{Proof of Corollary 2, Backwards Direction}
Since the proof proceeds analogously to the proof of \textbf{Theorem 1}, we will omit some of the details. See this for reference.



\subsection{Proof of Corollary 3}
\begin{proof}
First, we prove a generalization of \textbf{Proposition 1}.

\begin{claim}
For all $(\boldsymbol{x},\boldsymbol{A}$ satisfying $x_t \in A_t^C \neq \emptyset$,
\begin{align*}
    \rho_1(x_1,A_1^C)\prod_{t=2}^n \rho_t(x_t,A_t^C|A_{t-1}^C,x_{t-1};\cdots;A_1^C,x_1)=\sum_{\boldsymbol{D} \leq \boldsymbol{A}} M_{(\boldsymbol{x},\boldsymbol{D})}
\end{align*}
\end{claim}

Let $(L,\leq)$ be the product poset of $\{(2^{X_t},\subseteq)\}_{t=1}^n$ and define
\begin{align*}
    f(\boldsymbol{B}):=(-1)^{\sum_{t=1}^n |B_t|-|A_t^C|} \rho_1(x_1,B_1)\prod_{t=2}^n \rho_t(x_t,B_t|B_{t-1},x_{t-1};\cdots;B_1,x_1)
\end{align*}
and $F(\boldsymbol{D})=\sum_{\boldsymbol{B} \geq \boldsymbol{D}} f(\boldsymbol{B})$. By \textbf{Lemmas 2, 3, and 4}, 
\begin{align*}
    \rho_1(x_1,A_1^C)\prod_{t=2}^n \rho_t(x_t,A_t^C|A_{t-1}^C,x_{t-1};\cdots;A_1^C,x_1)=\sum_{\boldsymbol{B} \geq \boldsymbol{A}^C} (-1)^{\sum_{t=1}^n |B_t|-|A_t^C|} F(\boldsymbol{B})=\sum_{\boldsymbol{D} \leq \boldsymbol{A}} M_{(\boldsymbol{x},\boldsymbol{D})}
\end{align*}
since $(-1)^{\sum_{t=1}^n |D_t^C|-|A_t^C|} F(\boldsymbol{D}^C)=M_{(\boldsymbol{x},\boldsymbol{D})}$. \\ \\
Forwards direction: suppose $\mu$ is a SU representation of $\boldsymbol{\rho}^n$. By \textbf{Lemma 2},
\begin{align*}
    \rho_1(x_1,A_1^C)\prod_{t=2}^n \rho_t(x_t,A_t^C|A_{t-1}^C,x_{t-1};\cdots;A_1^C,x_1)=\sum_{\boldsymbol{B} \geq \boldsymbol{A}^C} \mu\big(E(\boldsymbol{x},\boldsymbol{B}^C)\big) \\
    \implies \mu\big(E(\boldsymbol{x},\boldsymbol{A})\big)=M_{(\boldsymbol{x},\boldsymbol{A})}
\end{align*}
Backwards direction: suppose $\mu\big(E(\boldsymbol{x},\boldsymbol{A})\big)=M_{(\boldsymbol{x},\boldsymbol{A})}$ for all $(\boldsymbol{x},\boldsymbol{A})$ satisfying $x_t \in A_t^C \neq \emptyset$. By \textbf{Claim 6},

\end{proof}
